# Supplementary material for: Visualization of Current-Driven Vortex Formation in High-$T_c$ Cuprate Superconductors
Source: arXiv:2511.19896 source file (2025-11-25)

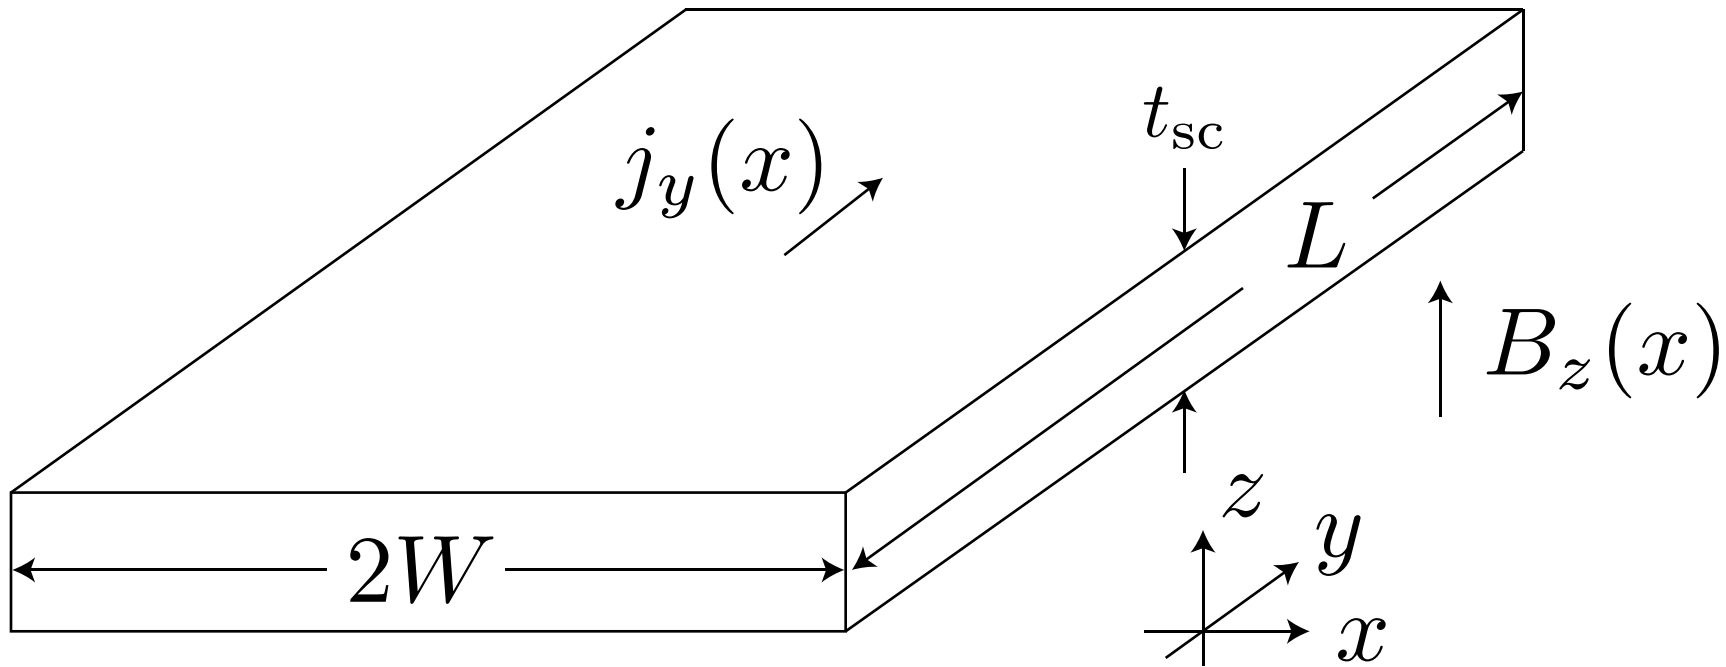

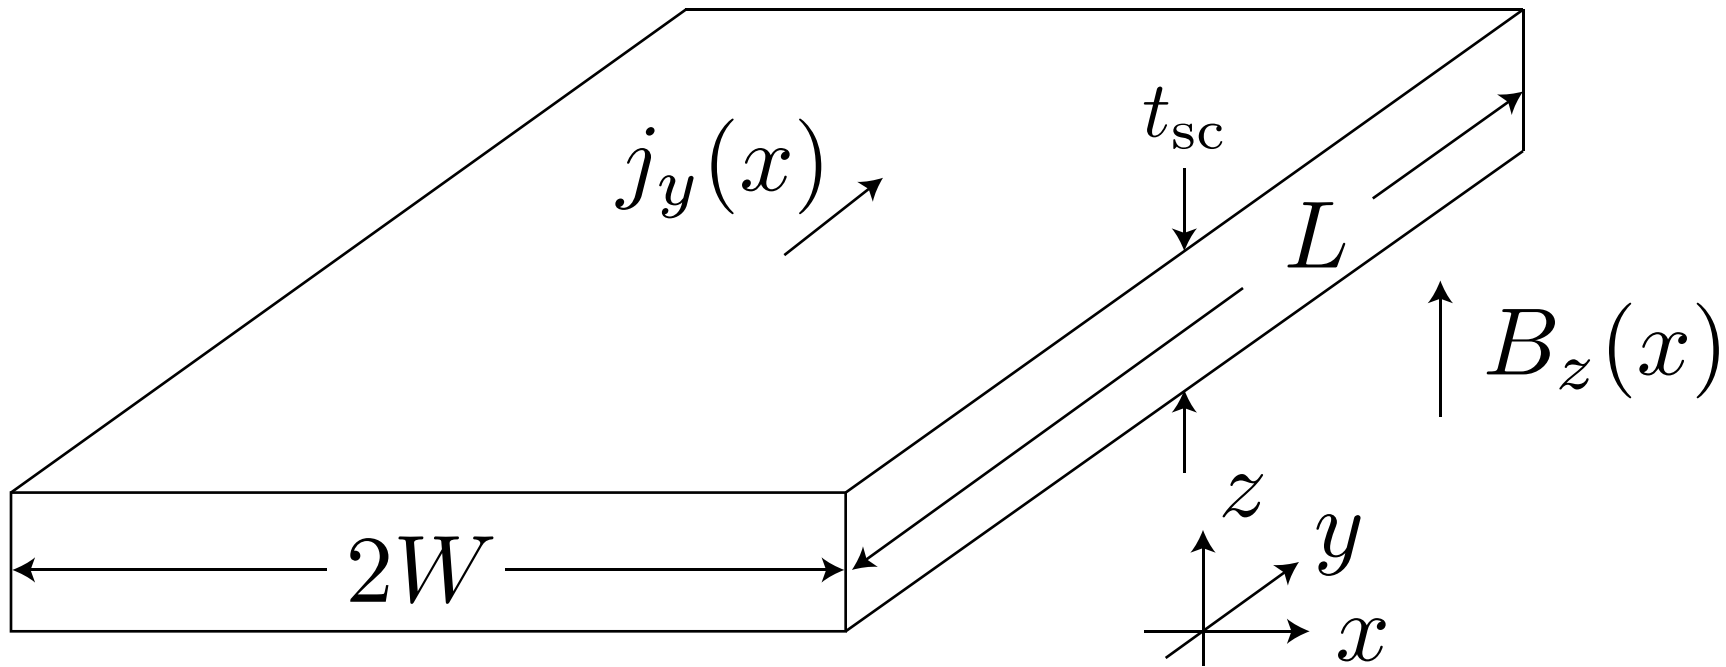

Supplement: Supplementary file 1 [file figS21.pdf]
